# Supplementary material for: Learning Robot Structure and Motion Embeddings using Graph Neural Networks
Source: arXiv:2109.07543 source file (2021-09-15)
Supplement: Supplementary file 1 [file appendix.tex]

% \section*{APPENDIX}

% Appendixes should appear before the acknowledgment.

\begin{figure*}
    \centering
    \includegraphics[width=1\linewidth]{images/temp/structure comparison.png}
    \caption{Caption}
\end{figure*}
\begin{figure*}
    \centering
    \includegraphics[width=1\linewidth]{images/temp/motion comparison.png}
    \caption{temp, compare mlp vs ours}
\end{figure*}

% \begin{figure}
%     \centering
%     \includegraphics[width=1\linewidth]{images/temp/mlp-structure.png}
%     \caption{structure embedding.
%     mlp, ours both: clusters w.r.t node;
%     mlp: dispersed within cluster;
%     ours: linear, can we say that 3,4 have similar robot structures
%     }
% \end{figure}

% \begin{figure}
%     \centering
%     \includegraphics[width=1\linewidth]{images/temp/mlp-motion.png}
%     \caption{motion embedding.
%     both: node feature, rather than num nodes. ;
%     mlp: ;
%     ours: single lengthy cluster
%     }
% \end{figure}

% \begin{figure}
%     \centering
%     \includegraphics[width=1\linewidth]{images/temp/tree-blanktree.png}
%     \caption{tree vs blank (motion)
%     blank distinguishes each data point better -- potential to 
%     }
% \end{figure}

% \section*{ACKNOWLEDGMENT}

% The preferred spelling of the word ÒacknowledgmentÓ in America is without an ÒeÓ after the ÒgÓ. Avoid the stilted expression, ÒOne of us (R. B. G.) thanks . . .Ó  Instead, try ÒR. B. G. thanksÓ. Put sponsor acknowledgments in the unnumbered footnote on the first page.
